# Supplementary material for: Universal Battery Performance and Degradation Model for Electric Aircraft
Source: arXiv:2008.01527 source file (2021-03-16)
Supplement: Supplementary file 1 [file SI.pdf]

# **Supplementary Information: Universal Battery Performance and Degradation Model for Electric Aircraft**

Alexander Bills<sup>1</sup>, Shashank Sripad<sup>1</sup>, William L. Fredericks<sup>1</sup>, Matthew Guttenberg<sup>1</sup>, Devin Charles<sup>2</sup>,  
Evan Frank<sup>2</sup>, Venkatasubramanian Viswanathan<sup>1,3</sup>

<sup>1</sup>*Department of Mechanical Engineering, Carnegie Mellon University, Pittsburgh, Pennsylvania, 15213, USA.*

<sup>2</sup>*A<sup>3</sup> by Airbus, Santa Clara, California, 95050, USA.*

<sup>3</sup>*Wilton E. Scott Institute for Energy Innovation, Carnegie Mellon University, Pittsburgh, Pennsylvania, 15213, USA.*

**This PDF includes:**

Supplementary Figures 1-4.

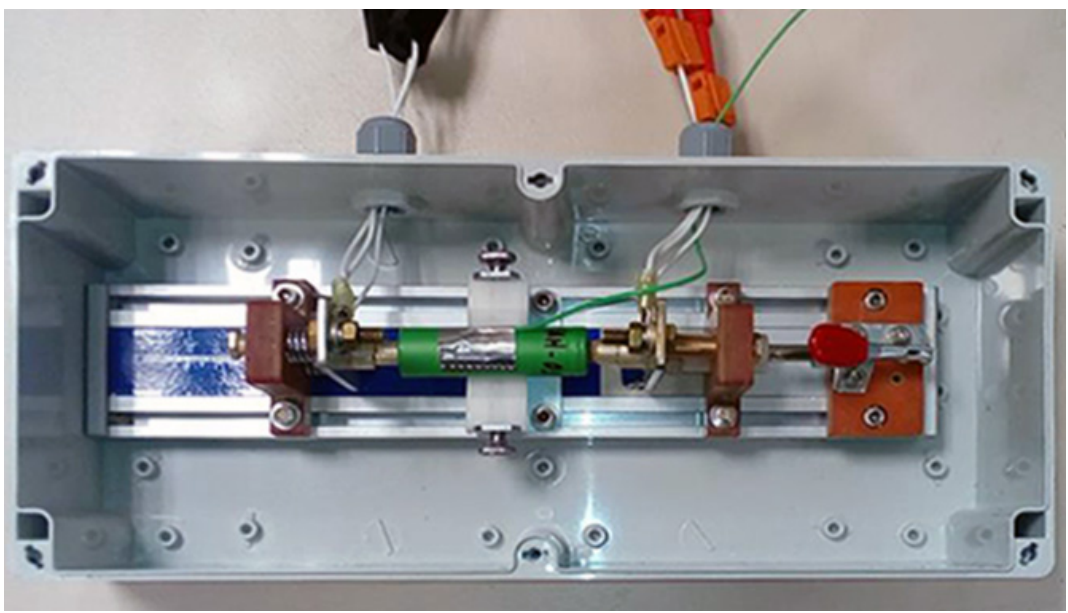

**Supplementary Figure 1: Cell holder and enclosure for battery performance dataset generation**

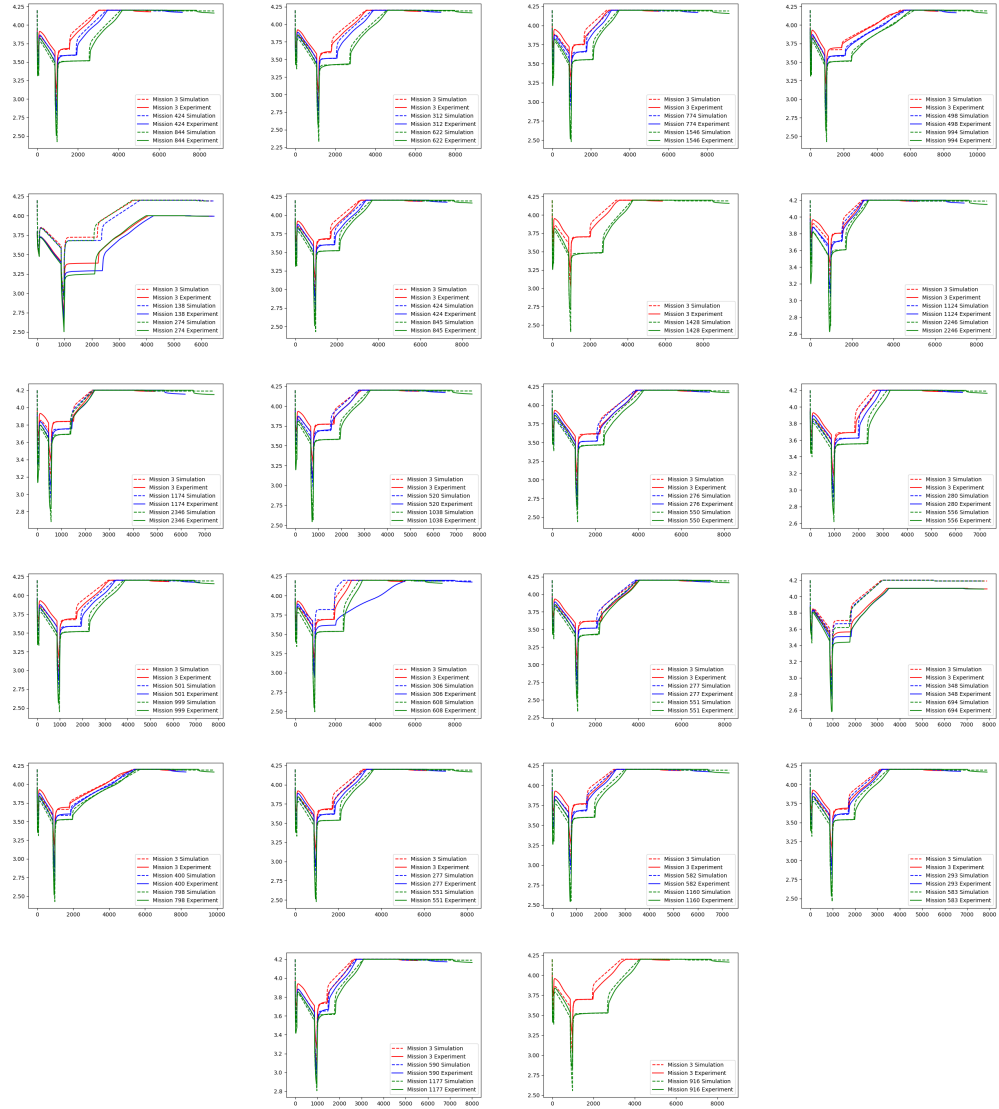

**Supplementary Figure 2: Voltage Figures: Voltage vs time for all cycles shown in this study.**

**Figures are ordered in order of their serial numbers (VAH1-30) from left to right and from top to bottom. 2 or 3 cycles from various stages of life are shown in each figure colored red, green, and blue, respectively, indicating early, mid, and late in life. Voltage tends to drop**

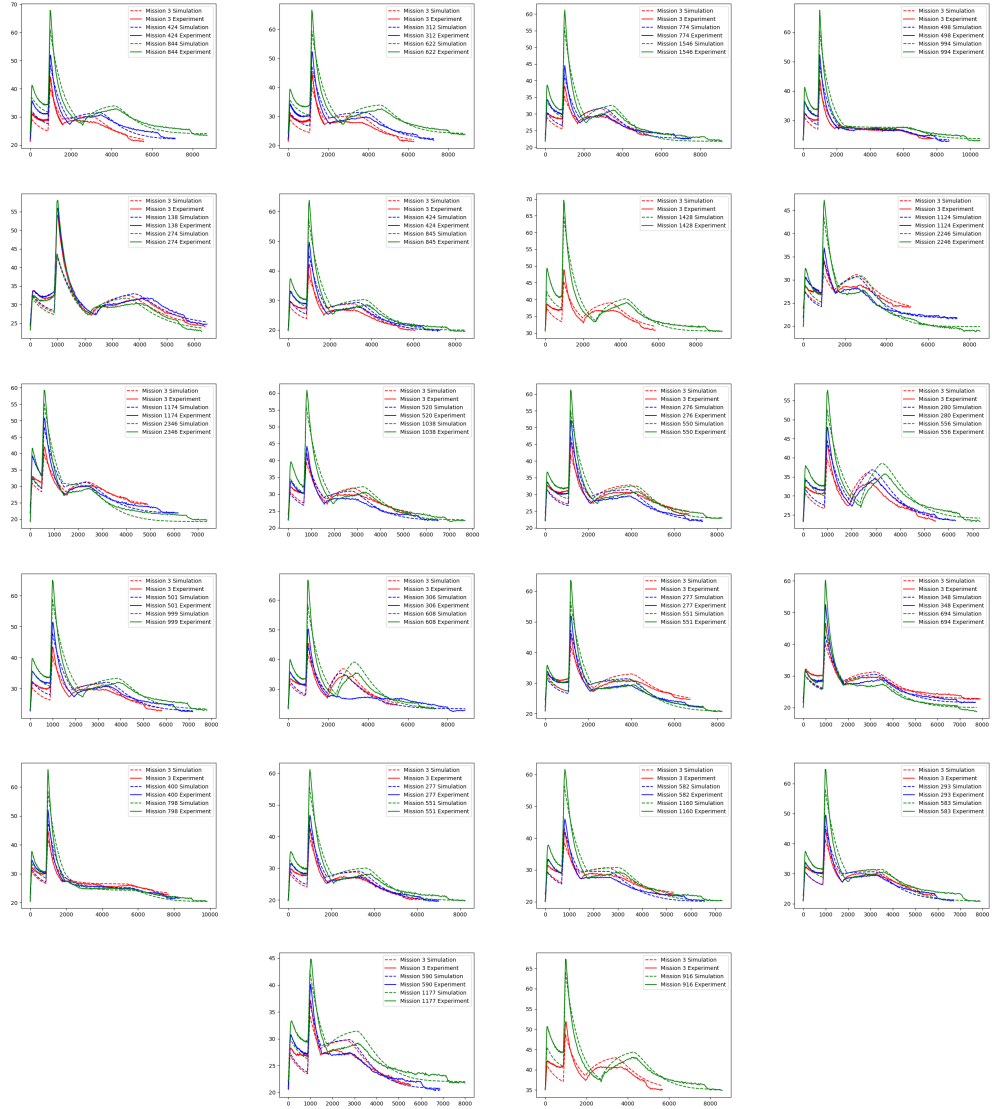

**Supplementary Figure 3: Temperature Figures: Temperature vs time for all cycles shown in this study. Figures are ordered in order of their serial numbers (VAH1-30) from left to right and from top to bottom. 2 or 3 cycles from various stages of life are shown in each figure colored red, green, and blue, respectively.**

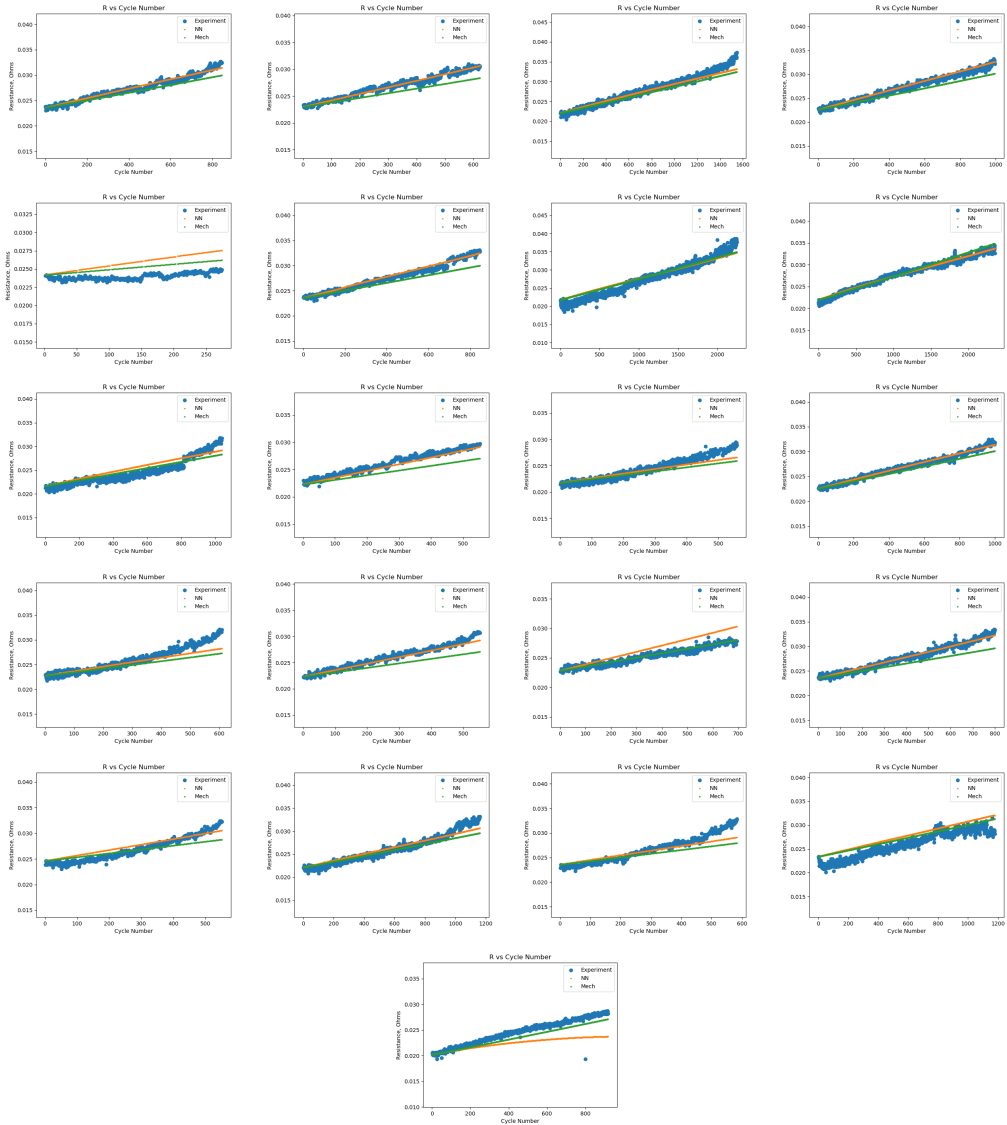

**Supplementary Figure 4: Resistance identified (optimized) values, and predicted values from the UBDM and mechanistic models for all cells in this study. Cells are ordered by their serial numbers from left to right and top to bottom.**

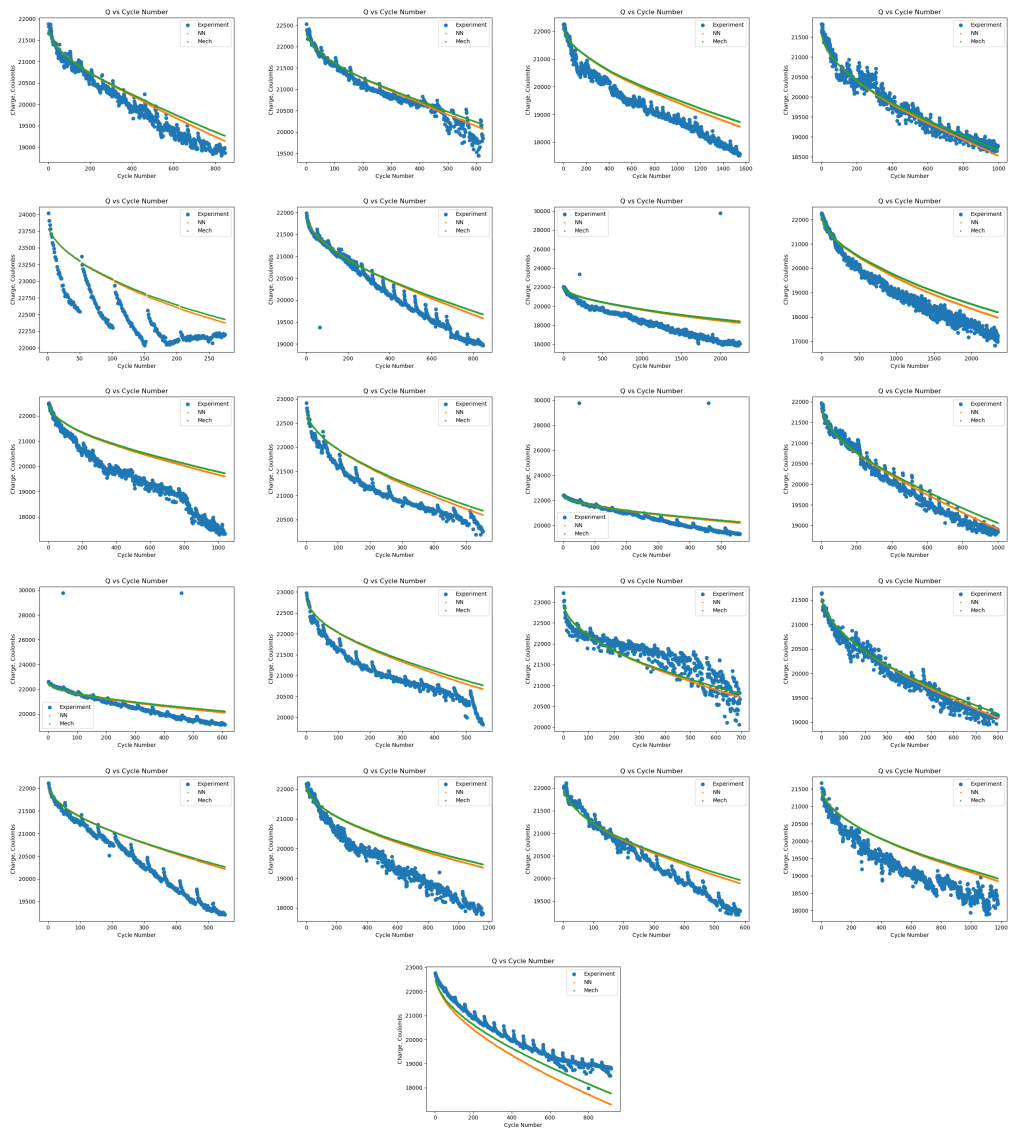

**Supplementary Figure 5: Charge identified (optimized) values, and predicted values from the UBDM and mechanistic models for all cells in this study. Cells are ordered by their serial numbers from left to right and top to bottom.**

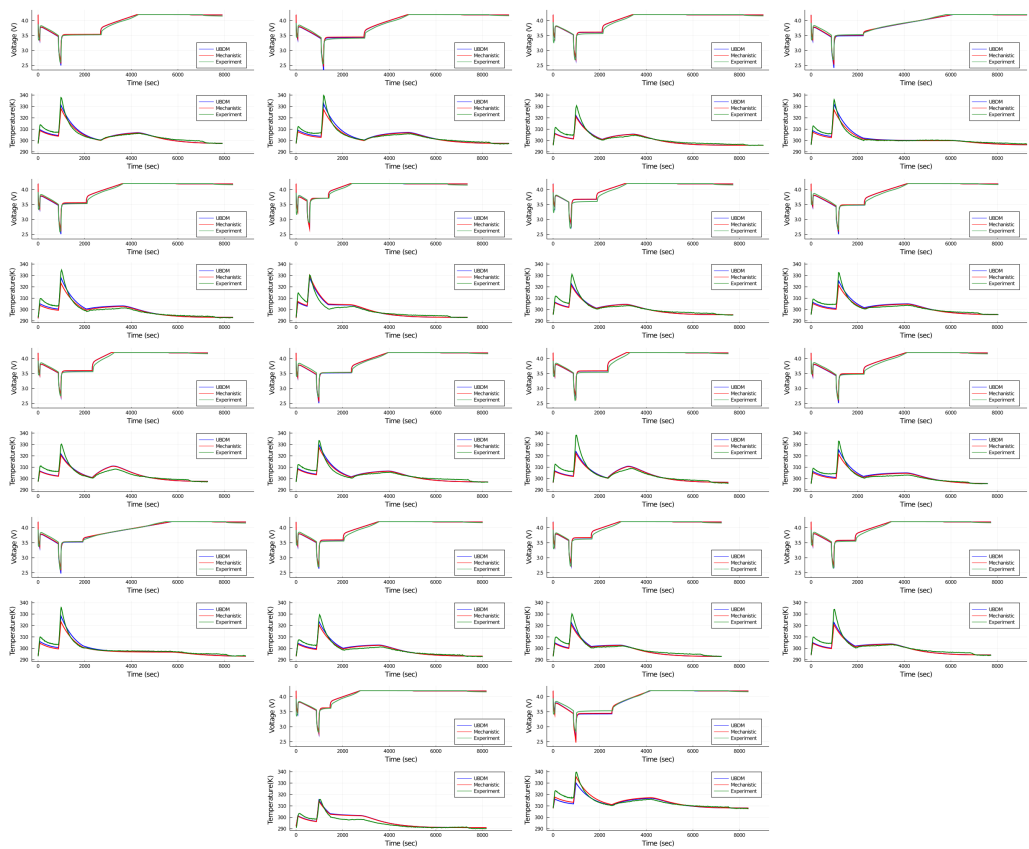

**Supplementary Figure 6: Voltage and Temperature vs Time for late cycles for all cells studied in this paper with true (experimental) values, UBDM predictions, and predictions from the mechanistic model. Cells are ordered in order of their serial number from left to right and top to bottom, with each subfigure having voltage on the top and temperature on the bottom.**

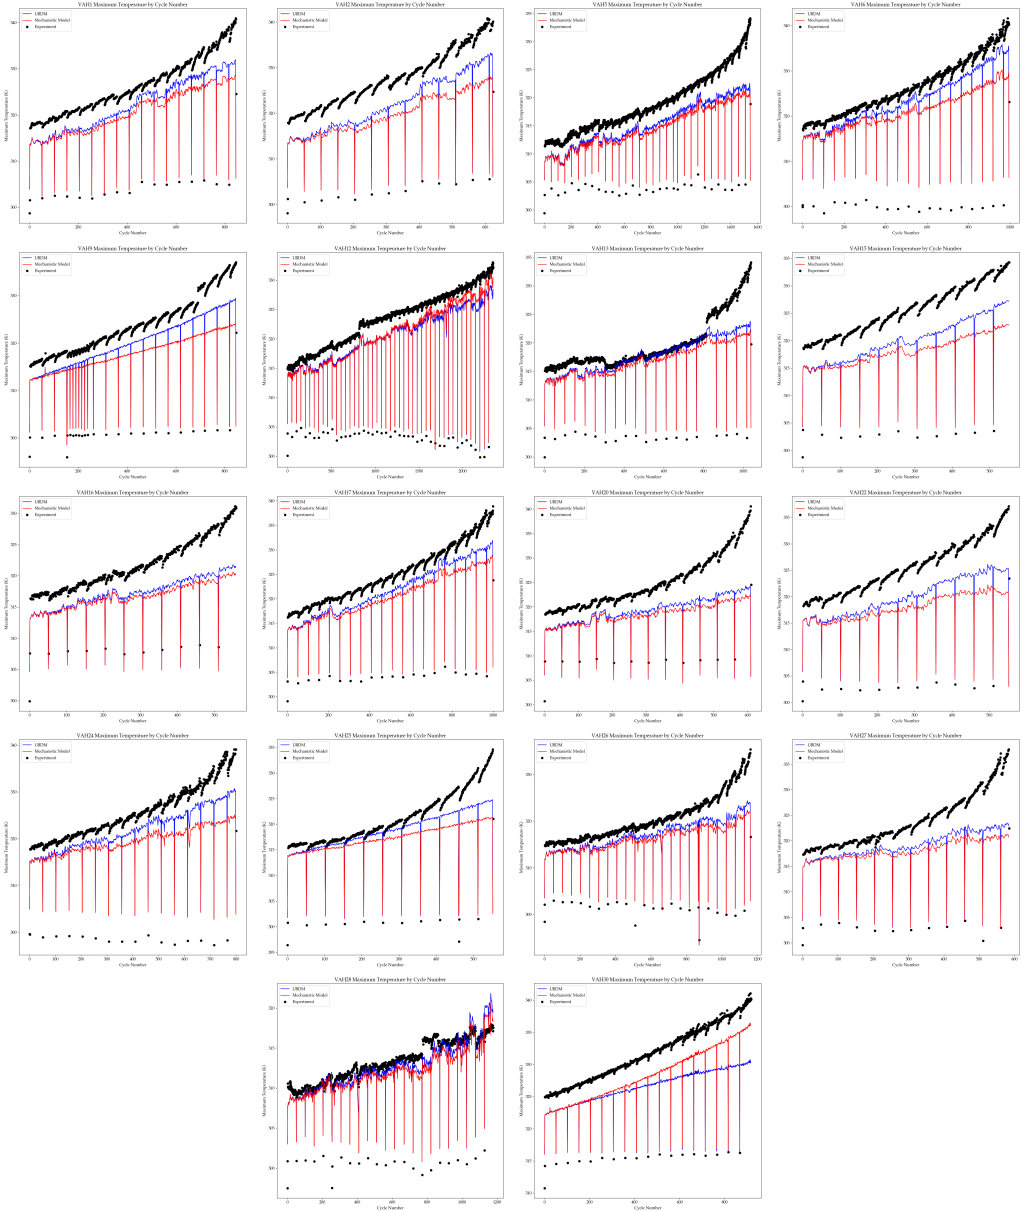

**Supplementary Figure 7: Maximum Temperature vs cycle number for all cycles considered in this study for the UBDM, the mechanistic model, and experimental results. In nearly all cases, the UBDM outperforms the mechanistic model (VAH30 is the only real exception, and this discrepancy can be explained by VAH30 being a part of the extrapolative set)**
